# Supplementary material for: A Unified Framework for Shot Type Classification Based on Subject Centric Lens
Source: arXiv:2008.03548 source file (2020-08-08)
Supplement: Supplementary file 1 [file supp.tex]

% !TEX root = ../main.tex

\clearpage
